# Supplementary material for: DensePhysNet: Learning Dense Physical Object Representations via Multi-step Dynamic Interactions
Source: arXiv:1906.03853 source file (2019-06-11)
Supplement: Supplementary file 1 [file appendix.tex]

\section{Appendix}
\subsection{Details on real-world experiment}
the setup
the object's material

\subsection{Details on background subtraction}
